# Supplementary material for: MEOW: MEMOry Supervised LLM Unlearning Via Inverted Facts
Source: arXiv:2409.11844 source file (2024-09-18)
Supplement: Supplementary file 1 [file analysis_setup.tex]

\section{Experimental Setup for Additional Analysis}

\subsection{Introduction to LLMs}
